# Supplementary material for: Subsampling (weighted smooth) empirical copula processes
Source: arXiv:1811.10957 source file (2023-01-31)
Supplement: Supplementary file 1 [file sub-supp.pdf]

# Supplementary material for “Subsampling (weighted smooth) empirical copula processes”

Ivan Kojadinovic[1] and Kristina Stemikovskaya[1,2]

[1]CNRS / Université de Pau et des Pays de l'Adour / E2S UPPA, Laboratoire de mathématiques et applications – IPRA, UMR 5142, B.P. 1155, 64013 Pau Cedex, France. E-mail: ivan.kojadinovic@univ-pau.fr
[2]Universidad del País Vasco, Intelligent Systems Group, Campus de Guipuzcoa, 20018 Donostia - San Sebastian, Spain. E-mail: kristina.stemikovskaya@ehu.eus

May 23, 2019

**Abstract**

This supplement contains additional simulation results for the empirical bootstrap, the multiplier bootstrap, subsampling and the $b$ out of $n$ bootstrap in the context of resampling the empirical copula processes in the case of i.i.d. observations.

The factors of the Monte Carlo experiments whose results are reported in this supplement are the family of the exchangeable copula (Clayton or Gumbel–Hougaard) from which i.i.d. observations are generated, the dimension $d \in \{2, 4\}$ of the copula, the value of Kendall's tau $\tau \in \{0.33, 0.66\}$ of the bivariate margins of the copula and the size $n \in \{100, 200, 400\}$ of the generated samples. Four resampling methods are considered: the classical empirical bootstrap, the multiplier bootstrap, subsampling and the $b$ out of $n$ bootstrap (of which the empirical bootstrap is a particular case). For all four methods, centering is used as explained in the manuscript. For subsampling and the $b$ out of $n$ bootstrap, the subsample size $b$ is taken to be in the set $\{\lfloor 0.1n \rfloor, \lfloor 0.28n \rfloor, \lfloor 0.50n \rfloor, \lfloor 0.75n \rfloor\}$. Subsampling is carried out first without and then with the finite population correction. The $b$ out of $n$ bootstrap is not carried out with the finite population correction since the latter has no justification in this case (and this would prevent the empirical bootstrap to arise as a particular case of the method for $b = n$).

Tables 1 and 5 report empirical mean squared errors (MSEs) for the empirical bootstrap and the multiplier bootstrap for $d$ equal 2 and 4, respectively.

Tables 2 and 6 report empirical MSEs for the $b$ out of $n$ bootstrap for $d$ equal 2 and 4, respectively.

Tables 3 and 7 report empirical MSEs for subsampling without the finite population correction for $d$ equal 2 and 4, respectively.

Tables 4 and 8 report empirical MSEs for subsampling with the finite population correction for $d$ equal 2 and 4, respectively.

The following empirical conclusions can be drawn:

- the multiplier bootstrap is uniformly better than the empirical bootstrap;
- for the $b$ out of $n$ bootstrap, the smallest empirical MSEs are obtained when $b$ is "small" compared to $n$, that is, when $b \in \{\lfloor 0.1n \rfloor, \lfloor 0.28n \rfloor\}$;
- for subsampling, the use of the finite population correction seems, overall, beneficial, although, for $d = 2$ and in the case of the estimation of covariances or high quantiles of Kolmogorov–Smirnov functionals, proceeding without the finite population correction might lead, overall, to slighty smaller empirical MSEs;
- the $b$ out of $n$ bootstrap leads, overall, to larger empirical MSEs than subsampling with the finite population correction;
- for subsampling with the finite population correction, choosing $b \in \{\lfloor 0.1n \rfloor, \lfloor 0.28n \rfloor\}$ leads, overall, to the smallest empirical MSEs ; for estimating high quantiles of Cramér–von Mises functionals, the choice $b = \lfloor 0.28n \rfloor$ seems better, overall; for estimating covariances or high quantiles of Kolmogorov–Smirnov functionals, the choice $b = \lfloor 0.1n \rfloor$ might be better, overall;
- with an appropriate choice of $b \in \{\lfloor 0.1n \rfloor, \lfloor 0.28n \rfloor\}$, the performance of subsampling with the finite population correction can, overall, match that of the multiplier bootstrap.

Table 1: Averages of the empirical MSEs ($\times 10^4$) of covariance estimators at the points $P = \{(i/3, j/3) : i, j = 1, 2\}$ (column $\overline{cov}$) and empirical MSEs ($\times 10^4$) of estimators of the 90% and 95%-quantiles of $KS(\hat{\mathbb{C}}_n)$ and $CvM(\hat{\mathbb{C}}_n)$ based on the **empirical bootstrap** (boot) and the **multiplier bootstrap** (mult) from i.i.d. samples of size $n$ generated from a **bivariate copula** $C$ with a Kendall's tau of $\tau$.

| Copula | $\tau$ | $n$ | method | $\overline{cov}$ | KS90 | KS95 | CvM90 | CvM95 |
|---|---|---|---|---|---|---|---|---|
| Clayton | 0.33 | 100 | boot | 1.307 | 154.680 | 127.228 | 2.600 | 3.251 |
| | | | mult | 0.489 | 14.127 | 8.240 | 0.349 | 0.597 |
| Clayton | 0.33 | 200 | boot | 0.675 | 62.282 | 67.004 | 1.023 | 1.315 |
| | | | mult | 0.269 | 6.884 | 8.063 | 0.189 | 0.338 |
| Clayton | 0.33 | 400 | boot | 0.338 | 29.184 | 36.912 | 0.484 | 0.589 |
| | | | mult | 0.180 | 4.289 | 6.496 | 0.110 | 0.193 |
| Clayton | 0.66 | 100 | boot | 1.007 | 141.490 | 206.733 | 1.992 | 2.598 |
| | | | mult | 0.350 | 11.561 | 18.857 | 0.204 | 0.321 |
| Clayton | 0.66 | 200 | boot | 0.510 | 67.644 | 88.481 | 0.710 | 0.909 |
| | | | mult | 0.188 | 9.423 | 14.600 | 0.127 | 0.199 |
| Clayton | 0.66 | 400 | boot | 0.255 | 25.198 | 30.003 | 0.271 | 0.351 |
| | | | mult | 0.148 | 4.412 | 6.280 | 0.061 | 0.098 |
| Gumbel–Hougaard | 0.33 | 100 | boot | 1.421 | 154.456 | 150.616 | 2.641 | 3.380 |
| | | | mult | 0.422 | 9.209 | 7.455 | 0.318 | 0.551 |
| Gumbel–Hougaard | 0.33 | 200 | boot | 0.687 | 55.431 | 72.926 | 1.099 | 1.358 |
| | | | mult | 0.290 | 3.553 | 6.662 | 0.166 | 0.278 |
| Gumbel–Hougaard | 0.33 | 400 | boot | 0.349 | 30.861 | 37.968 | 0.477 | 0.618 |
| | | | mult | 0.148 | 4.360 | 6.561 | 0.109 | 0.190 |
| Gumbel–Hougaard | 0.66 | 100 | boot | 1.115 | 183.148 | 254.828 | 2.143 | 2.887 |
| | | | mult | 0.311 | 11.986 | 17.690 | 0.182 | 0.276 |
| Gumbel–Hougaard | 0.66 | 200 | boot | 0.522 | 90.053 | 100.719 | 0.763 | 0.981 |
| | | | mult | 0.220 | 9.849 | 10.166 | 0.094 | 0.135 |
| Gumbel–Hougaard | 0.66 | 400 | boot | 0.264 | 32.451 | 46.191 | 0.274 | 0.348 |
| | | | mult | 0.113 | 4.264 | 7.298 | 0.049 | 0.075 |

Table 2: Averages of the empirical MSEs ($\times 10^4$) of covariance estimators at the points $P = \{(i/3, j/3) : i, j = 1, 2\}$ (column $\overline{cov}$) and empirical MSEs ($\times 10^4$) of estimators of the 90% and 95%-quantiles of $KS(\hat{\mathbb{C}}_n)$ and $CvM(\hat{\mathbb{C}}_n)$ based on the $b$ **out of** $n$ **bootstrap** with subsample size $b$ from i.i.d. samples of size $n$ generated from a **bivariate copula** $C$ with a Kendall's tau of $\tau$.

| Copula | $\tau$ | $n$ | $b$ | $\overline{cov}$ | KS90 | KS95 | CvM90 | CvM95 |
|---|---|---|---|---|---|---|---|---|
| Clayton | 0.33 | 100 | 10 | 0.381 | 43.435 | 47.684 | 1.447 | 3.425 |
| | | | 28 | 0.542 | 60.730 | 43.817 | 0.495 | 0.660 |
| | | | 50 | 0.870 | 98.706 | 75.102 | 1.789 | 2.361 |
| | | | 75 | 1.166 | 124.004 | 100.044 | 1.889 | 2.347 |
| Clayton | 0.33 | 200 | 20 | 0.238 | 12.475 | 13.626 | 0.450 | 0.752 |
| | | | 56 | 0.321 | 23.284 | 24.902 | 0.381 | 0.563 |
| | | | 100 | 0.412 | 35.831 | 38.954 | 0.669 | 0.945 |
| | | | 150 | 0.570 | 49.115 | 53.030 | 0.827 | 1.140 |
| Clayton | 0.33 | 400 | 40 | 0.110 | 5.967 | 7.790 | 0.175 | 0.268 |
| | | | 112 | 0.165 | 9.807 | 13.036 | 0.181 | 0.262 |
| | | | 200 | 0.231 | 15.951 | 20.281 | 0.296 | 0.389 |
| | | | 300 | 0.292 | 22.345 | 28.825 | 0.390 | 0.496 |
| Clayton | 0.66 | 100 | 10 | 0.651 | 99.250 | 199.825 | 3.374 | 7.506 |
| | | | 28 | 0.540 | 72.589 | 138.257 | 1.291 | 2.183 |
| | | | 50 | 0.732 | 95.747 | 156.886 | 1.664 | 2.515 |
| | | | 75 | 0.881 | 116.345 | 178.069 | 1.702 | 2.319 |
| Clayton | 0.66 | 200 | 20 | 0.302 | 29.349 | 68.281 | 0.865 | 2.055 |
| | | | 56 | 0.269 | 29.761 | 47.041 | 0.437 | 0.724 |
| | | | 100 | 0.319 | 41.517 | 59.366 | 0.537 | 0.760 |
| | | | 150 | 0.421 | 55.056 | 74.661 | 0.621 | 0.820 |
| Clayton | 0.66 | 400 | 40 | 0.092 | 5.728 | 11.539 | 0.189 | 0.459 |
| | | | 112 | 0.124 | 8.339 | 10.978 | 0.139 | 0.221 |
| | | | 200 | 0.173 | 13.835 | 16.793 | 0.190 | 0.270 |
| | | | 300 | 0.219 | 19.359 | 23.074 | 0.231 | 0.310 |
| Gumbel–Hougaard | 0.33 | 100 | 10 | 0.426 | 44.841 | 72.868 | 1.414 | 3.719 |
| | | | 28 | 0.626 | 61.296 | 58.925 | 0.464 | 0.654 |
| | | | 50 | 0.934 | 97.687 | 92.358 | 1.804 | 2.466 |
| | | | 75 | 1.267 | 122.160 | 116.750 | 1.906 | 2.437 |
| Gumbel–Hougaard | 0.33 | 200 | 20 | 0.238 | 9.706 | 18.392 | 0.480 | 0.782 |
| | | | 56 | 0.324 | 19.566 | 28.746 | 0.410 | 0.564 |
| | | | 100 | 0.428 | 30.856 | 42.582 | 0.723 | 0.936 |
| | | | 150 | 0.576 | 44.095 | 59.164 | 0.928 | 1.151 |
| Gumbel–Hougaard | 0.33 | 400 | 40 | 0.108 | 7.150 | 8.866 | 0.192 | 0.278 |
| | | | 112 | 0.161 | 11.126 | 14.332 | 0.194 | 0.272 |
| | | | 200 | 0.222 | 17.890 | 22.597 | 0.314 | 0.408 |
| | | | 300 | 0.288 | 25.058 | 30.590 | 0.400 | 0.502 |
| Gumbel–Hougaard | 0.66 | 100 | 10 | 0.709 | 150.123 | 258.156 | 3.712 | 8.297 |
| | | | 28 | 0.600 | 106.090 | 186.428 | 1.329 | 2.326 |
| | | | 50 | 0.772 | 134.864 | 204.730 | 1.797 | 2.841 |
| | | | 75 | 0.991 | 152.884 | 221.143 | 1.791 | 2.536 |
| Gumbel–Hougaard | 0.66 | 200 | 20 | 0.250 | 54.147 | 84.919 | 0.984 | 2.287 |
| | | | 56 | 0.267 | 46.619 | 59.018 | 0.475 | 0.847 |
| | | | 100 | 0.338 | 59.802 | 67.536 | 0.576 | 0.836 |
| | | | 150 | 0.444 | 75.434 | 84.141 | 0.673 | 0.902 |
| Gumbel–Hougaard | 0.66 | 400 | 40 | 0.095 | 12.122 | 26.288 | 0.222 | 0.561 |
| | | | 112 | 0.125 | 12.849 | 22.153 | 0.147 | 0.237 |
| | | | 200 | 0.174 | 18.777 | 28.907 | 0.193 | 0.273 |
| | | | 300 | 0.223 | 25.999 | 37.909 | 0.236 | 0.316 |

Table 3: Averages of the empirical MSEs ($\times 10^4$) of covariance estimators at the points $P = \{(i/3, j/3) : i, j = 1, 2\}$ (column $\overline{cov}$) and empirical MSEs ($\times 10^4$) of estimators of the 90% and 95%-quantiles of $KS(\hat{\mathbb{C}}_n)$ and $CvM(\hat{\mathbb{C}}_n)$ based on **subsampling** with subsample size $b$ from i.i.d. samples of size $n$ generated from a **bivariate copula** $C$ with a Kendall's tau of $\tau$. Subsampling is carried out **without the finite population correction**.

| Copula | $\tau$ | $n$ | $b$ | $\overline{cov}$ | KS90 | KS95 | CvM90 | CvM95 |
|---|---|---|---|---|---|---|---|---|
| Clayton | 0.33 | 100 | 10 | 0.306 | 5.598 | 9.955 | 0.185 | 0.232 |
| | | | 28 | 0.555 | 18.822 | 48.740 | 1.800 | 3.033 |
| | | | 50 | 1.516 | 99.999 | 177.792 | 3.505 | 5.877 |
| | | | 75 | 3.876 | 423.493 | 625.049 | 9.584 | 15.557 |
| Clayton | 0.33 | 200 | 20 | 0.138 | 5.267 | 8.234 | 0.181 | 0.276 |
| | | | 56 | 0.513 | 32.794 | 44.893 | 1.307 | 2.135 |
| | | | 100 | 1.733 | 156.524 | 200.634 | 4.021 | 6.476 |
| | | | 150 | 4.216 | 546.998 | 682.627 | 10.147 | 16.025 |
| Clayton | 0.33 | 400 | 40 | 0.147 | 4.642 | 5.507 | 0.175 | 0.324 |
| | | | 112 | 0.596 | 45.478 | 52.643 | 1.375 | 2.345 |
| | | | 200 | 1.868 | 190.705 | 225.335 | 4.338 | 7.099 |
| | | | 300 | 4.497 | 625.993 | 746.869 | 10.603 | 16.970 |
| Clayton | 0.66 | 100 | 10 | 0.156 | 10.812 | 23.251 | 0.541 | 1.513 |
| | | | 28 | 0.136 | 21.387 | 17.068 | 0.220 | 0.341 |
| | | | 50 | 0.355 | 83.235 | 85.825 | 0.456 | 0.854 |
| | | | 75 | 0.911 | 289.929 | 318.893 | 1.283 | 2.239 |
| Clayton | 0.66 | 200 | 20 | 0.096 | 4.495 | 4.513 | 0.108 | 0.363 |
| | | | 56 | 0.136 | 23.747 | 26.152 | 0.156 | 0.254 |
| | | | 100 | 0.397 | 94.492 | 112.513 | 0.489 | 0.840 |
| | | | 150 | 0.999 | 328.284 | 389.502 | 1.320 | 2.151 |
| Clayton | 0.66 | 400 | 40 | 0.046 | 6.886 | 6.283 | 0.038 | 0.079 |
| | | | 112 | 0.147 | 35.639 | 44.839 | 0.175 | 0.280 |
| | | | 200 | 0.443 | 127.636 | 160.946 | 0.560 | 0.893 |
| | | | 300 | 1.089 | 399.159 | 489.081 | 1.426 | 2.208 |
| Gumbel–Hougaard | 0.33 | 100 | 10 | 0.269 | 5.457 | 8.212 | 0.171 | 0.196 |
| | | | 28 | 0.491 | 23.793 | 45.959 | 1.881 | 3.078 |
| | | | 50 | 1.412 | 113.171 | 173.325 | 3.638 | 5.965 |
| | | | 75 | 3.651 | 443.481 | 606.532 | 9.678 | 15.413 |
| Gumbel–Hougaard | 0.33 | 200 | 20 | 0.128 | 8.038 | 6.995 | 0.159 | 0.250 |
| | | | 56 | 0.479 | 41.564 | 44.709 | 1.261 | 2.116 |
| | | | 100 | 1.655 | 173.227 | 197.187 | 3.939 | 6.429 |
| | | | 150 | 4.051 | 577.403 | 673.634 | 9.995 | 15.876 |
| Gumbel–Hougaard | 0.33 | 400 | 40 | 0.130 | 3.886 | 5.058 | 0.156 | 0.282 |
| | | | 112 | 0.551 | 43.592 | 50.848 | 1.341 | 2.261 |
| | | | 200 | 1.784 | 186.243 | 223.264 | 4.286 | 6.923 |
| | | | 300 | 4.317 | 617.239 | 739.210 | 10.510 | 16.629 |
| Gumbel–Hougaard | 0.66 | 100 | 10 | 0.155 | 22.251 | 33.386 | 0.623 | 1.582 |
| | | | 28 | 0.118 | 13.247 | 15.019 | 0.193 | 0.290 |
| | | | 50 | 0.317 | 64.730 | 73.114 | 0.422 | 0.769 |
| | | | 75 | 0.838 | 247.633 | 286.860 | 1.203 | 2.047 |
| Gumbel–Hougaard | 0.66 | 200 | 20 | 0.061 | 6.859 | 5.501 | 0.124 | 0.391 |
| | | | 56 | 0.117 | 15.222 | 22.173 | 0.135 | 0.208 |
| | | | 100 | 0.355 | 73.434 | 103.718 | 0.447 | 0.744 |
| | | | 150 | 0.919 | 277.480 | 361.665 | 1.225 | 1.931 |
| Gumbel–Hougaard | 0.66 | 400 | 40 | 0.037 | 4.335 | 2.264 | 0.030 | 0.076 |
| | | | 112 | 0.118 | 26.682 | 27.063 | 0.159 | 0.243 |
| | | | 200 | 0.384 | 109.814 | 122.793 | 0.521 | 0.803 |
| | | | 300 | 0.984 | 357.382 | 412.832 | 1.338 | 2.005 |

Table 4: Averages of the empirical MSEs ($\times 10^4$) of covariance estimators at the points $P = \{(i/3, j/3) : i, j = 1, 2\}$ (column $\overline{cov}$) and empirical MSEs ($\times 10^4$) of estimators of the 90% and 95%-quantiles of $KS(\hat{\mathbb{C}}_n)$ and $CvM(\hat{\mathbb{C}}_n)$ based on **subsampling** with subsample size $b$ from i.i.d. samples of size $n$ generated from a **bivariate copula** $C$ with a Kendall's tau of $\tau$. Subsampling is carried out **with the finite population correction**.

| Copula | $\tau$ | $n$ | $b$ | $\overline{cov}$ | KS90 | KS95 | CvM90 | CvM95 |
|---|---|---|---|---|---|---|---|---|
| Clayton | 0.33 | 100 | 10 | 0.311 | 17.165 | 6.877 | 0.429 | 0.888 |
| | | | 28 | 0.456 | 35.083 | 19.755 | 0.266 | 0.450 |
| | | | 50 | 0.987 | 96.223 | 72.141 | 1.245 | 1.674 |
| | | | 75 | 2.558 | 251.329 | 221.191 | 2.813 | 3.437 |
| Clayton | 0.33 | 200 | 20 | 0.185 | 7.692 | 4.877 | 0.231 | 0.379 |
| | | | 56 | 0.295 | 17.051 | 17.996 | 0.246 | 0.393 |
| | | | 100 | 0.522 | 43.434 | 46.441 | 0.609 | 0.828 |
| | | | 150 | 1.303 | 124.859 | 139.397 | 1.596 | 2.060 |
| Clayton | 0.33 | 400 | 40 | 0.104 | 3.536 | 5.093 | 0.128 | 0.218 |
| | | | 112 | 0.168 | 8.225 | 11.347 | 0.137 | 0.202 |
| | | | 200 | 0.309 | 22.608 | 29.184 | 0.330 | 0.436 |
| | | | 300 | 0.700 | 66.292 | 82.085 | 0.837 | 1.020 |
| Clayton | 0.66 | 100 | 10 | 0.323 | 33.951 | 59.220 | 0.997 | 2.569 |
| | | | 28 | 0.325 | 22.470 | 41.905 | 0.175 | 0.306 |
| | | | 50 | 0.697 | 63.342 | 93.951 | 0.545 | 0.698 |
| | | | 75 | 1.756 | 200.167 | 272.336 | 1.247 | 1.474 |
| Clayton | 0.66 | 200 | 20 | 0.186 | 10.766 | 16.702 | 0.264 | 0.773 |
| | | | 56 | 0.218 | 16.548 | 23.211 | 0.150 | 0.243 |
| | | | 100 | 0.387 | 41.741 | 53.558 | 0.291 | 0.375 |
| | | | 150 | 0.948 | 121.714 | 155.470 | 0.699 | 0.864 |
| Clayton | 0.66 | 400 | 40 | 0.071 | 3.505 | 4.003 | 0.079 | 0.212 |
| | | | 112 | 0.121 | 6.287 | 7.321 | 0.071 | 0.112 |
| | | | 200 | 0.225 | 17.743 | 20.659 | 0.144 | 0.197 |
| | | | 300 | 0.517 | 59.307 | 72.280 | 0.355 | 0.460 |
| Gumbel–Hougaard | 0.33 | 100 | 10 | 0.296 | 12.405 | 6.838 | 0.361 | 0.806 |
| | | | 28 | 0.413 | 27.345 | 19.729 | 0.253 | 0.417 |
| | | | 50 | 0.873 | 81.406 | 71.531 | 1.115 | 1.486 |
| | | | 75 | 2.335 | 230.596 | 223.313 | 2.659 | 3.244 |
| Gumbel–Hougaard | 0.33 | 200 | 20 | 0.163 | 5.302 | 4.660 | 0.221 | 0.338 |
| | | | 56 | 0.263 | 11.430 | 17.181 | 0.226 | 0.325 |
| | | | 100 | 0.462 | 34.276 | 46.081 | 0.608 | 0.779 |
| | | | 150 | 1.258 | 107.395 | 136.794 | 1.597 | 1.930 |
| Gumbel–Hougaard | 0.33 | 400 | 40 | 0.093 | 4.121 | 5.204 | 0.124 | 0.204 |
| | | | 112 | 0.151 | 8.388 | 11.483 | 0.135 | 0.198 |
| | | | 200 | 0.278 | 22.842 | 27.966 | 0.322 | 0.418 |
| | | | 300 | 0.671 | 64.710 | 77.927 | 0.807 | 0.961 |
| Gumbel–Hougaard | 0.66 | 100 | 10 | 0.322 | 54.244 | 75.089 | 1.114 | 2.646 |
| | | | 28 | 0.298 | 30.794 | 46.605 | 0.171 | 0.298 |
| | | | 50 | 0.592 | 75.123 | 96.216 | 0.535 | 0.651 |
| | | | 75 | 1.587 | 220.806 | 276.498 | 1.234 | 1.383 |
| Gumbel–Hougaard | 0.66 | 200 | 20 | 0.134 | 20.266 | 22.394 | 0.298 | 0.810 |
| | | | 56 | 0.182 | 22.032 | 21.688 | 0.139 | 0.213 |
| | | | 100 | 0.335 | 51.477 | 51.175 | 0.277 | 0.338 |
| | | | 150 | 0.884 | 143.715 | 154.120 | 0.711 | 0.827 |
| Gumbel–Hougaard | 0.66 | 400 | 40 | 0.067 | 4.651 | 11.311 | 0.079 | 0.220 |
| | | | 112 | 0.108 | 8.105 | 12.858 | 0.064 | 0.097 |
| | | | 200 | 0.203 | 20.187 | 28.784 | 0.132 | 0.167 |
| | | | 300 | 0.483 | 65.490 | 85.812 | 0.341 | 0.414 |

Table 5: Empirical MSEs ($\times 10^4$) of estimators of the 90% and 95%-quantiles of $KS(\hat{\mathbb{C}}_n)$ and $CvM(\hat{\mathbb{C}}_n)$ based on the **empirical bootstrap** (boot) and the **multiplier bootstrap** (mult) from i.i.d. samples of size $n$ generated from a **four-variate copula** $C$ whose bivariate margins have a Kendall's tau of $\tau$.

| Copula | $\tau$ | $n$ | method | KS90 | KS95 | CvM90 | CvM95 |
|---|---|---|---|---|---|---|---|
| Clayton | 0.33 | 100 | boot | 98.520 | 102.514 | 2.506 | 3.638 |
| | | | mult | 9.160 | 8.868 | 0.742 | 1.638 |
| Clayton | 0.33 | 200 | boot | 40.014 | 50.519 | 1.593 | 2.489 |
| | | | mult | 3.877 | 6.372 | 0.485 | 1.064 |
| Clayton | 0.33 | 400 | boot | 32.767 | 26.451 | 0.865 | 1.441 |
| | | | mult | 6.028 | 4.131 | 0.389 | 0.801 |
| Clayton | 0.66 | 100 | boot | 118.640 | 137.810 | 3.918 | 5.473 |
| | | | mult | 20.605 | 26.047 | 0.731 | 1.255 |
| Clayton | 0.66 | 200 | boot | 51.547 | 62.367 | 1.702 | 2.391 |
| | | | mult | 11.101 | 14.815 | 0.359 | 0.632 |
| Clayton | 0.66 | 400 | boot | 38.687 | 46.820 | 0.839 | 1.201 |
| | | | mult | 10.387 | 14.080 | 0.261 | 0.449 |
| Gumbel–Hougaard | 0.33 | 100 | boot | 188.556 | 175.659 | 3.215 | 4.142 |
| | | | mult | 29.856 | 24.716 | 0.408 | 0.802 |
| Gumbel–Hougaard | 0.33 | 200 | boot | 81.068 | 94.692 | 1.671 | 2.227 |
| | | | mult | 13.311 | 17.800 | 0.305 | 0.606 |
| Gumbel–Hougaard | 0.33 | 400 | boot | 43.746 | 40.056 | 1.002 | 1.467 |
| | | | mult | 8.785 | 8.213 | 0.252 | 0.488 |
| Gumbel–Hougaard | 0.66 | 100 | boot | 194.247 | 277.658 | 5.283 | 7.174 |
| | | | mult | 36.899 | 59.200 | 1.048 | 1.566 |
| Gumbel–Hougaard | 0.66 | 200 | boot | 95.895 | 119.951 | 2.318 | 3.190 |
| | | | mult | 20.374 | 28.491 | 0.556 | 0.876 |
| Gumbel–Hougaard | 0.66 | 400 | boot | 52.553 | 63.284 | 1.005 | 1.404 |
| | | | mult | 13.400 | 17.570 | 0.316 | 0.526 |

Table 6: Empirical MSEs ($\times 10^4$) of estimators of the 90% and 95%-quantiles of $KS(\hat{\mathbb{C}}_n)$ and $CvM(\hat{\mathbb{C}}_n)$ based on the $b$ **out** $n$ **bootstrap** with subsample size $b$ from i.i.d. samples of size $n$ generated from a **four-variate copula** $C$ whose bivariate margins have a Kendall's tau of $\tau$.

| Copula | $\tau$ | $n$ | $b$ | KS90 | KS95 | CvM90 | CvM95 |
|---|---|---|---|---|---|---|---|
| Clayton | 0.33 | 100 | 10 | 6.135 | 5.009 | 0.340 | 0.569 |
| | | | 28 | 21.968 | 18.684 | 0.542 | 1.492 |
| | | | 50 | 47.635 | 47.907 | 1.382 | 2.005 |
| | | | 75 | 74.108 | 76.752 | 2.003 | 2.987 |
| Clayton | 0.33 | 200 | 20 | 3.075 | 4.305 | 0.343 | 0.596 |
| | | | 56 | 7.381 | 10.020 | 0.435 | 0.838 |
| | | | 100 | 18.024 | 24.095 | 0.917 | 1.392 |
| | | | 150 | 29.388 | 37.810 | 1.290 | 1.931 |
| Clayton | 0.33 | 400 | 40 | 4.035 | 2.683 | 0.247 | 0.546 |
| | | | 112 | 9.705 | 6.346 | 0.339 | 0.661 |
| | | | 200 | 17.343 | 12.700 | 0.514 | 0.878 |
| | | | 300 | 24.689 | 18.864 | 0.657 | 1.126 |
| Clayton | 0.66 | 100 | 10 | 19.225 | 44.079 | 6.867 | 15.539 |
| | | | 28 | 39.156 | 52.819 | 1.762 | 3.349 |
| | | | 50 | 66.245 | 79.682 | 3.002 | 4.835 |
| | | | 75 | 93.367 | 109.464 | 3.382 | 4.915 |
| Clayton | 0.66 | 200 | 20 | 13.102 | 20.468 | 1.764 | 4.990 |
| | | | 56 | 16.015 | 22.334 | 0.824 | 1.523 |
| | | | 100 | 27.691 | 35.251 | 1.199 | 1.896 |
| | | | 150 | 39.469 | 49.056 | 1.449 | 2.109 |
| Clayton | 0.66 | 400 | 40 | 9.045 | 15.392 | 0.527 | 1.418 |
| | | | 112 | 14.579 | 19.424 | 0.413 | 0.730 |
| | | | 200 | 22.470 | 27.767 | 0.563 | 0.873 |
| | | | 300 | 30.830 | 37.951 | 0.715 | 1.057 |
| Gumbel–Hougaard | 0.33 | 100 | 10 | 16.291 | 8.938 | 0.250 | 0.234 |
| | | | 28 | 48.763 | 34.677 | 0.180 | 0.558 |
| | | | 50 | 100.853 | 84.369 | 1.585 | 2.062 |
| | | | 75 | 145.218 | 131.464 | 2.345 | 3.023 |
| Gumbel–Hougaard | 0.33 | 200 | 20 | 6.896 | 8.890 | 0.182 | 0.273 |
| | | | 56 | 22.141 | 24.198 | 0.253 | 0.363 |
| | | | 100 | 41.629 | 48.543 | 0.825 | 1.105 |
| | | | 150 | 63.879 | 75.606 | 1.301 | 1.722 |
| Gumbel–Hougaard | 0.33 | 400 | 40 | 5.383 | 4.543 | 0.170 | 0.277 |
| | | | 112 | 13.364 | 10.411 | 0.247 | 0.394 |
| | | | 200 | 23.454 | 20.032 | 0.565 | 0.799 |
| | | | 300 | 33.561 | 30.371 | 0.767 | 1.124 |
| Gumbel–Hougaard | 0.66 | 100 | 10 | 64.464 | 146.865 | 4.196 | 10.454 |
| | | | 28 | 63.928 | 116.474 | 1.291 | 2.256 |
| | | | 50 | 114.513 | 176.777 | 3.514 | 5.314 |
| | | | 75 | 153.704 | 225.503 | 4.361 | 6.156 |
| Gumbel–Hougaard | 0.66 | 200 | 20 | 25.294 | 44.491 | 1.253 | 3.139 |
| | | | 56 | 32.054 | 46.301 | 0.863 | 1.402 |
| | | | 100 | 53.209 | 70.815 | 1.473 | 2.158 |
| | | | 150 | 75.071 | 95.549 | 1.887 | 2.633 |
| Gumbel–Hougaard | 0.66 | 400 | 40 | 14.238 | 22.149 | 0.389 | 0.877 |
| | | | 112 | 19.857 | 26.337 | 0.399 | 0.662 |
| | | | 200 | 29.745 | 36.496 | 0.631 | 0.944 |
| | | | 300 | 42.030 | 50.378 | 0.823 | 1.167 |

Table 7: Empirical MSEs ($\times 10^4$) of estimators of the 90% and 95%-quantiles of $KS(\hat{\mathbb{C}}_n)$ and $CvM(\hat{\mathbb{C}}_n)$ based on **subsampling** with subsample size $b$ from i.i.d. samples of size $n$ generated from a **four-variate copula** $C$ whose bivariate margins have a Kendall's tau of $\tau$. Subsampling is carried out **without the finite population correction**.

| Copula | $\tau$ | $n$ | $b$ | KS90 | KS95 | CvM90 | CvM95 |
|---|---|---|---|---|---|---|---|
| Clayton | 0.33 | 100 | 10 | 6.796 | 16.453 | 0.899 | 2.375 |
| | | | 28 | 59.190 | 86.621 | 7.982 | 14.459 |
| | | | 50 | 267.808 | 349.977 | 16.075 | 27.159 |
| | | | 75 | 967.832 | 1207.217 | 40.696 | 67.273 |
| Clayton | 0.33 | 200 | 20 | 16.305 | 16.130 | 0.829 | 1.987 |
| | | | 56 | 93.504 | 109.506 | 5.660 | 10.287 |
| | | | 100 | 367.170 | 432.846 | 17.211 | 29.309 |
| | | | 150 | 1174.369 | 1391.231 | 42.485 | 70.933 |
| Clayton | 0.33 | 400 | 40 | 7.223 | 17.848 | 0.934 | 2.043 |
| | | | 112 | 83.649 | 124.503 | 6.083 | 10.750 |
| | | | 200 | 364.757 | 489.227 | 18.919 | 32.154 |
| | | | 300 | 1194.641 | 1524.041 | 44.846 | 74.960 |
| Clayton | 0.66 | 100 | 10 | 10.092 | 8.480 | 1.820 | 5.680 |
| | | | 28 | 43.460 | 59.912 | 0.741 | 1.312 |
| | | | 50 | 178.438 | 239.844 | 1.795 | 3.391 |
| | | | 75 | 629.586 | 811.034 | 5.060 | 9.014 |
| Clayton | 0.66 | 200 | 20 | 10.256 | 9.783 | 0.390 | 1.422 |
| | | | 56 | 63.904 | 76.480 | 0.630 | 1.052 |
| | | | 100 | 240.314 | 297.731 | 1.947 | 3.340 |
| | | | 150 | 765.779 | 946.556 | 5.284 | 8.747 |
| Clayton | 0.66 | 400 | 40 | 7.235 | 7.899 | 0.136 | 0.352 |
| | | | 112 | 53.445 | 65.608 | 0.627 | 1.010 |
| | | | 200 | 234.806 | 290.026 | 2.147 | 3.496 |
| | | | 300 | 774.543 | 953.965 | 5.550 | 8.805 |
| Gumbel–Hougaard | 0.33 | 100 | 10 | 6.046 | 24.699 | 0.463 | 1.457 |
| | | | 28 | 53.233 | 105.452 | 6.178 | 10.984 |
| | | | 50 | 246.317 | 376.322 | 12.873 | 21.287 |
| | | | 75 | 958.312 | 1294.777 | 33.878 | 54.479 |
| Gumbel–Hougaard | 0.33 | 200 | 20 | 12.797 | 23.912 | 0.542 | 1.345 |
| | | | 56 | 85.169 | 109.904 | 4.831 | 8.410 |
| | | | 100 | 356.749 | 441.479 | 14.556 | 23.793 |
| | | | 150 | 1206.013 | 1471.531 | 36.721 | 58.989 |
| Gumbel–Hougaard | 0.33 | 400 | 40 | 11.935 | 24.711 | 0.535 | 1.159 |
| | | | 112 | 96.446 | 141.905 | 4.718 | 7.949 |
| | | | 200 | 412.336 | 544.094 | 15.644 | 25.341 |
| | | | 300 | 1332.026 | 1686.944 | 38.073 | 60.894 |
| Gumbel–Hougaard | 0.66 | 100 | 10 | 12.919 | 39.254 | 0.752 | 2.350 |
| | | | 28 | 43.669 | 43.932 | 1.528 | 2.595 |
| | | | 50 | 164.528 | 187.045 | 3.345 | 5.906 |
| | | | 75 | 601.859 | 702.959 | 9.510 | 15.816 |
| Gumbel–Hougaard | 0.66 | 200 | 20 | 7.814 | 7.691 | 0.213 | 0.550 |
| | | | 56 | 52.048 | 64.277 | 1.260 | 2.087 |
| | | | 100 | 211.019 | 259.976 | 3.944 | 6.501 |
| | | | 150 | 711.922 | 868.192 | 10.446 | 16.546 |
| Gumbel–Hougaard | 0.66 | 400 | 40 | 5.364 | 6.588 | 0.199 | 0.284 |
| | | | 112 | 53.015 | 67.173 | 1.354 | 2.161 |
| | | | 200 | 235.537 | 295.432 | 4.461 | 7.026 |
| | | | 300 | 781.318 | 955.661 | 11.217 | 17.240 |

Table 8: Empirical MSEs ($\times 10^4$) of estimators of the 90% and 95%-quantiles of $KS(\hat{\mathbb{C}}_n)$ and $CvM(\hat{\mathbb{C}}_n)$ based on **subsampling** with subsample size $b$ from i.i.d. samples of size $n$ generated from a **four-variate copula** $C$ whose bivariate margins have a Kendall's tau of $\tau$. Subsampling is carried out **with the finite population correction**.

| Copula | $\tau$ | $n$ | $b$ | KS90 | KS95 | CvM90 | CvM95 |
|---|---|---|---|---|---|---|---|
| Clayton | 0.33 | 100 | 10 | 7.298 | 4.318 | 0.507 | 0.749 |
| | | | 28 | 30.013 | 26.299 | 0.616 | 1.435 |
| | | | 50 | 93.631 | 93.883 | 2.814 | 4.449 |
| | | | 75 | 273.148 | 293.762 | 7.642 | 11.175 |
| Clayton | 0.33 | 200 | 20 | 2.722 | 5.008 | 0.400 | 0.627 |
| | | | 56 | 10.825 | 14.168 | 0.597 | 1.055 |
| | | | 100 | 37.756 | 46.842 | 1.605 | 2.488 |
| | | | 150 | 127.013 | 152.246 | 4.160 | 5.965 |
| Clayton | 0.33 | 400 | 40 | 4.395 | 2.967 | 0.270 | 0.533 |
| | | | 112 | 12.750 | 8.944 | 0.391 | 0.778 |
| | | | 200 | 32.187 | 25.157 | 0.872 | 1.401 |
| | | | 300 | 87.712 | 79.230 | 2.186 | 3.178 |
| Clayton | 0.66 | 100 | 10 | 19.220 | 26.599 | 3.481 | 9.804 |
| | | | 28 | 36.505 | 40.037 | 0.734 | 1.346 |
| | | | 50 | 91.820 | 97.484 | 2.272 | 3.303 |
| | | | 75 | 262.238 | 286.175 | 5.620 | 7.634 |
| Clayton | 0.66 | 200 | 20 | 10.257 | 15.615 | 0.977 | 3.038 |
| | | | 56 | 16.403 | 21.543 | 0.557 | 0.995 |
| | | | 100 | 42.322 | 49.767 | 1.197 | 1.767 |
| | | | 150 | 130.849 | 151.957 | 2.938 | 4.081 |
| Clayton | 0.66 | 400 | 40 | 8.101 | 11.472 | 0.341 | 0.953 |
| | | | 112 | 16.022 | 20.349 | 0.345 | 0.585 |
| | | | 200 | 34.226 | 41.284 | 0.657 | 0.976 |
| | | | 300 | 91.836 | 107.354 | 1.535 | 2.191 |
| Gumbel–Hougaard | 0.33 | 100 | 10 | 21.133 | 8.457 | 0.273 | 0.287 |
| | | | 28 | 49.702 | 34.073 | 0.204 | 0.503 |
| | | | 50 | 154.097 | 133.931 | 2.991 | 3.944 |
| | | | 75 | 416.243 | 417.194 | 9.768 | 13.040 |
| Gumbel–Hougaard | 0.33 | 200 | 20 | 6.881 | 7.275 | 0.200 | 0.305 |
| | | | 56 | 23.878 | 27.144 | 0.333 | 0.512 |
| | | | 100 | 69.602 | 80.104 | 1.677 | 2.315 |
| | | | 150 | 201.254 | 232.119 | 4.898 | 6.473 |
| Gumbel–Hougaard | 0.33 | 400 | 40 | 5.046 | 5.035 | 0.172 | 0.290 |
| | | | 112 | 15.414 | 12.527 | 0.328 | 0.518 |
| | | | 200 | 37.840 | 34.608 | 0.930 | 1.364 |
| | | | 300 | 109.670 | 109.538 | 2.660 | 3.672 |
| Gumbel–Hougaard | 0.66 | 100 | 10 | 20.350 | 91.241 | 2.055 | 5.424 |
| | | | 28 | 43.480 | 67.115 | 0.640 | 0.966 |
| | | | 50 | 127.701 | 169.528 | 2.997 | 3.847 |
| | | | 75 | 377.835 | 476.087 | 8.208 | 10.331 |
| Gumbel–Hougaard | 0.66 | 200 | 20 | 20.365 | 25.634 | 0.654 | 1.679 |
| | | | 56 | 25.094 | 32.365 | 0.614 | 0.908 |
| | | | 100 | 70.309 | 83.685 | 1.563 | 2.074 |
| | | | 150 | 213.341 | 256.239 | 4.192 | 5.449 |
| Gumbel–Hougaard | 0.66 | 400 | 40 | 10.516 | 15.175 | 0.272 | 0.567 |
| | | | 112 | 18.689 | 22.401 | 0.342 | 0.537 |
| | | | 200 | 42.004 | 46.930 | 0.733 | 1.004 |
| | | | 300 | 119.128 | 139.437 | 1.946 | 2.569 |
